# Supplementary material for: Ab-initio transport theory for the intrinsic spin Hall effect applied to 5$d$ metals
Source: arXiv:2401.01658 source file (2024-04-29)
Supplement: Supplementary file 1 [file suppmat_v3.pdf]

# Supplemental Material for "*Ab-initio* transport theory for the intrinsic spin Hall effect applied to $5d$ metals"

Akash Bajaj,[1] Reena Gupta,[1] Ilya V. Tokatly,[2,3,4] Stefano Sanvito,[1] and Andrea Droghetti[1]

[1]*School of Physics and CRANN, Trinity College Dublin, Dublin 2, Ireland*

[2]*Nano-Bio Spectroscopy Group and European Theoretical Spectroscopy Facility (ETSF), Departamento de Polímeros y Materiales Avanzados: Física, Química y Tecnología, Universidad del País Vasco (UPV/EHU), Av. Tolosa 72, 20018 San Sebastián, Spain*

[3]*Donostia International Physics Center (DIPC), 20018 Donostia-San Sebastián, Spain*

[4]*IKERBASQUE, Basque Foundation for Science, 48009 Bilbao, Spain*

(Dated: April 29, 2024)

# Table of Contents

**Dependence of the spin Hall current on the number of k-points** 3

**SHC for supercells of different transverse sizes** 3

**Dependence of the SHC on the k-point sampling** 3

**Device structures** 4

**Variation in spin-Hall conductivity with Fermi level position in Ta** 5

**Spin hall current for W.** 6

**Spin hall current for Ir.** 7

**Spin hall current for Au.** 8

### Dependence of the spin Hall current on the number of k-points

TABLE S1: Spin Hall current in fcc Pt for different **k**-point grids. All calculations were carried out for a central region with 10 atomic layers at an applied bias voltage equal to 0.10 V.

| **k-point grid** ($k_x \times k_y \times 1$) | **spin Hall current,** $I_{\rm SH}$ (eV) |
|---|---|
| $11 \times 11 \times 1$ | $2.76 \times 10^{-2}$ |
| $13 \times 13 \times 1$ | $5.11 \times 10^{-2}$ |
| $15 \times 15 \times 1$ | $2.21 \times 10^{-2}$ |
| $19 \times 19 \times 1$ | $4.01 \times 10^{-2}$ |
| $21 \times 21 \times 1$ | $4.37 \times 10^{-2}$ |
| $31 \times 31 \times 1$ | $4.40 \times 10^{-2}$ |

### SHC for supercells of different transverse sizes

TABLE S2: SHC of fcc Pt for two supercells of different transverse sizes and 10 layers along the transport direction. $n_x$ and $n_y$ indicate the unit cell repetitions along the periodic $x$ and $y$ directions, respectively. The SHC is extracted from the spin current $I_x^y$.

| **Supercell transverse size** ($n_x \times n_y$) | **k-point grid** ($k_x \times k_y \times 1$) | **SHC** [$(\Omega\text{cm})^{-1}$)] |
|---|---|---|
| $1 \times 1$ | $20 \times 20 \times 1$ | 1620 |
| $2 \times 1$ | $10 \times 20 \times 1$ | 1750 |

### Dependence of the SHC on the k-point sampling

TABLE S3: Dependence of the SHC of fcc Pt on the **k**-point grid.

| **k-point grid** ($k_x \times k_y \times 1$) | **SHC** [$(\Omega\text{cm})^{-1}$] |
|---|---|
| $21 \times 21 \times 1$ | 1410 |
| $31 \times 31 \times 1$ | 1512 |

**Device structures**

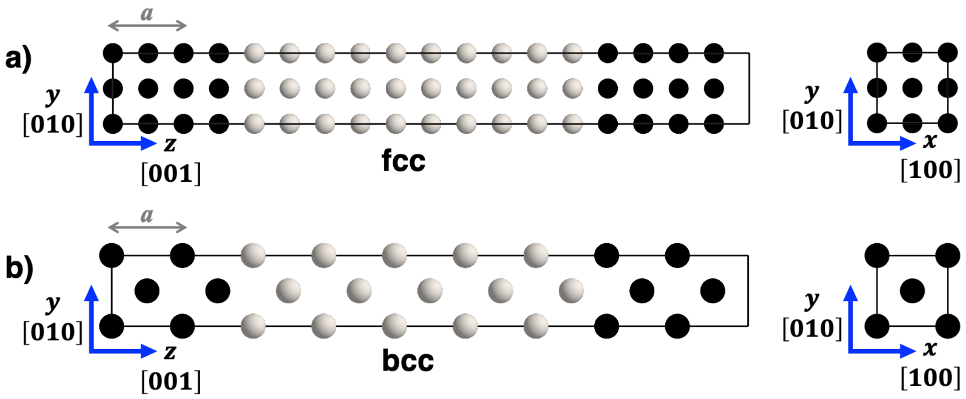


FIG. S1: Typical systems studied in the DFT+NEGF calculations. (a) and (b) are for materials with fcc and bcc structures, respectively. The leads and the central region are made of the same material. However, for distinguishing between the different parts of the system, atoms in central region are in grey, whereas atoms in the leads are in black. Only the systems with ten atomic layers in the central region are shown, although systems up to 40 layers were considered, as discussed in the main text. A Cartesian reference frame is introduced so that longitudinal transport is defined along the $z$ Cartesian direction, which is aligned with the [001] crystallographic direction. On the other hand, transverse spin transport is along the $x$ and $y$ Cartesian axes, which are oriented parallel to the [100] and [010] crystallographic directions, respectively. The materials' lattice constant parameters, $a$, are 3.306 Å (Ta), 3.152 Å (W), 3.838 Å (Ir), 3.924 Å (Pt), and 4.080 Å (Au).

### Variation in spin-Hall conductivity with Fermi level position in Ta

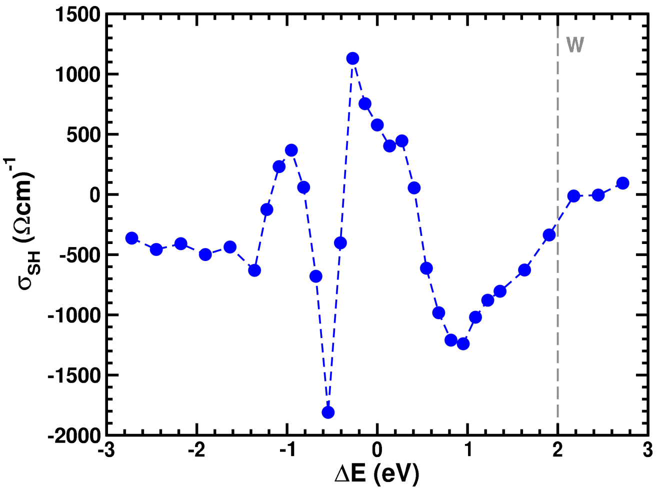


FIG. S2: SHC, $\sigma_{\mathrm{SH}}$, of Ta as a function of the Fermi energy position. Here $\Delta E$ is the position of $E_{\mathrm{F}}$ measured from the neutrality point, $\Delta E = 0$ (the true system Fermi energy). The vertical gray dashed line indicates the Fermi level corresponding to W.

**Spin hall current for W.**

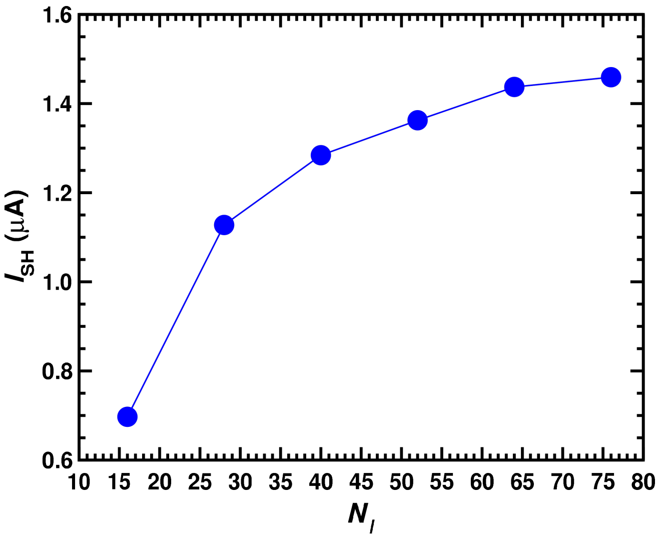


FIG. S3: Spin Hall current, $I_{\mathrm{SH}}$, at $V = 0.09$ V, as a function of the number of atomic layers, $N_l$, in the central region for W.

**Spin hall current for Ir.**

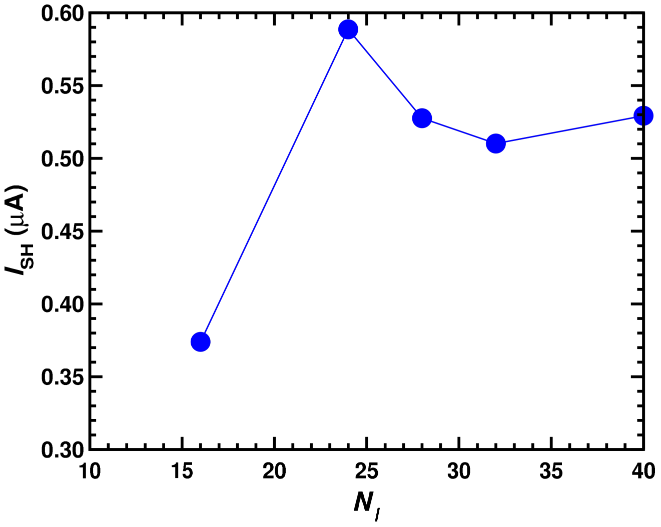


FIG. S4: Spin Hall current, $I_{\rm SH}$, at $V = 0.05$ V, as a function of the number of atomic layers, $N_l$, in the central region for Ir.

**Spin hall current for Au.**

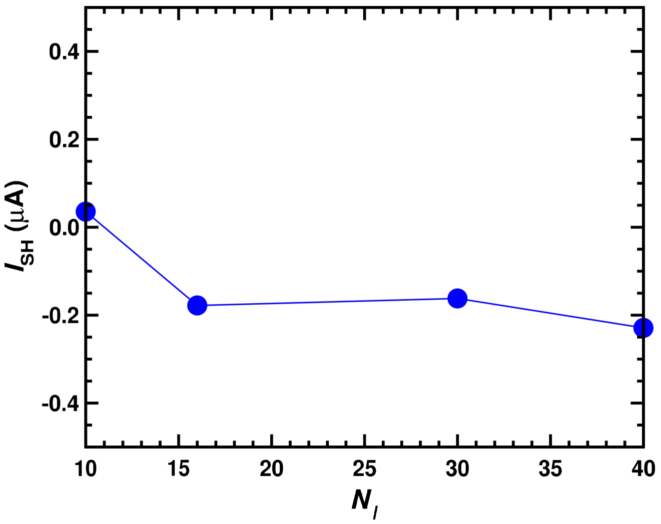


FIG. S5: Spin Hall current, $I_{\mathrm{SH}}$, at $V = 0.1$ V, as a function of the number of atomic layers, $N_l$, in the central region for Au.
